# Supplementary material for: Probabilistically Robust Learning: Balancing Average- and Worst-case Performance
Source: arXiv:2202.01136 source file (2022-06-07)
Supplement: Supplementary file 1 [file further-related-work.tex]

\section{Further related work}

\paragraph{Connections to risk.}

\begin{itemize}
    \item Connections to randomized smoothing~\cite{cohen2019certified,salman2019provably,kumar2020certifying}
    \item Frameworks that go between the average- and worst-case: Theory:~\cite{fawzi2016robustness} 
    \item Neither of the works in~\cite{rice2021robustness} or~\cite{li2020tilted,li2021tilted} minimize \emph{coherent} risk metrics; neither have interpretable parameters
    \item stochastic optimization, infinite-dimensional optimization~\cite{hsieh2019finding,vitt2019risk}, and statistical learning with risk measures
    
    \item In contrast to~\cite{curi2019adaptive} (and many of the works above), we do not wrap CVaR around $\Prob$; we wrap it around $\Prob_\Delta$.
    
    \item Applications to fairness~\cite{williamson2019fairness}
    
    \item Generalizing to out-of-distribution data
    
    \item Approximating/discretizing infinite-dimensional optimization problems~\cite{devolder2010solving}
    \item VaR and CVaR optimization.  Main reference is~\cite{nemirovski2007convex}; talks about CVaR being ``tightest convex inner-approximation''.
    \item Duality for constrained statistical problems~\cite{chamon2020empirical,chamon2020probably}; universal approximation~\cite{kratsios2021universal}
    \item and statistical learning with coherent measures of risk~\cite{takeda2009robust,khezeli2017risk,vitt2019risk,curi2019adaptive,kalogerias2020noisy,soma2020statistical}.
\end{itemize}

\paragraph{Connecting~\eqref{eq:p-cvar} to the conditional value-at-risk.}  As its label suggests, the constraint in~\eqref{eq:p-cvar} is equivalent to the well-known conditional value-at-risk (CVaR) metric.
This metric has been widely studied in the control~\cite{tsiamis2020risk,lindemann2021reactive}, reinforcement learning~\cite{chow2015risk,huang2017risk,chow2017risk}, and optimization~\cite{rockafellar2000optimization,rockafellar2002conditional,ghaoui2003worst} literature.  And while several recent works, including~\cite{takeda2009robust,vitt2019risk,soma2020statistical,curi2019adaptive,kalogerias2020noisy,khezeli2017risk}, have studied CVaR in a statistical supervised learning setting, this metric has not received widespread attention in the context of deep learning.
